# Supplementary material for: Minimal Adversarial Examples for Deep Learning on 3D Point Clouds
Source: arXiv:2008.12066 source file (2021-09-17)
Supplement: Supplementary file 1 [file supp_main.tex]

\begin{table*}[t]
\small
\begin{center}
\begin{tabular}{l|c|cc|c}
\toprule
& Success Rate & Chamfer Distance & Hausdorff Distance & \# Points\\
\midrule
Perturbation $\lambda 1$=0 & 99.67 & $2.06 \times {10^{-3}}$ & $4.58 \times {10^{-2}}$ & 536\\
Perturbation $\lambda 2$=0 & 98.53 & $9.03 \times {10^{-4}}$ & $3.61 \times {10^{-1}}$ & 6\\
Addition $\lambda 1$=0 & 98.62 & $8.46 \times {10^{-4}}$ & $4.75 \times {10^{-2}}$ & 986\\
Addition $\lambda 2$=0 & 99.03 & $1.19 \times {10^{-3}}$ & $4.22 \times {10^{-1}}$ & 6\\
\bottomrule 
\end{tabular}
\centerline{(a) ModelNet40}
\newline
\newline
\begin{tabular}{l|c|cc|c}
\toprule
& Success Rate & Chamfer Distance & Hausdorff Distance & \# Points\\
\midrule 
Perturbation $\lambda 1$=0 & 99.29 & $1.72 \times {10^{-3}}$ & $3.55 \times {10^{-2}}$ & 542\\
Perturbation $\lambda 2$=0 & 97.16 & $6.59 \times {10^{-4}}$ & $3.22 \times {10^{-1}}$ & 7\\
Addition $\lambda 1$=0 & 98.81 & $6.73 \times {10^{-4}}$ & $3.44 \times {10^{-2}}$ & 983\\
Addition $\lambda 2$=0 & 98.81 & $7.32 \times {10^{-4}}$ & $3.45 \times {10^{-1}}$ & 6\\
\bottomrule
\end{tabular}
\centerline{(b) ScanObjectNN}
\caption{Comparison of point sparsity and object perceptibility in generating adversarial examples in point perturbation and point addition on both synthetic and real-world data.}
\label{table:Lambda_variation}
\end{center}%
\end{table*}

\begin{table*}[t]
\small
\begin{center}
\begin{tabular}{l|c|cc|c}
\toprule
& Success Rate & Chamfer Distance & Hausdorff Distance & \# Points\\
\midrule
Chamfer & 98.35 & $2.94 \times {10^{-4}}$ & $9.03 \times {10^{-2}}$ & 42\\
Hausdorff & 89.38 & $1.55 \times {10^{-4}}$ & $1.88 \times {10^{-2}}$ & 36\\
\bottomrule 
\end{tabular}
\centerline{(a) Perturbation attack on ModelNet40}
\newline
\newline
\begin{tabular}{l|c|cc|c}
\toprule
& Success Rate & Chamfer Distance & Hausdorff Distance & \# Points\\
\midrule
Chamfer & 97.71 & $3.36 \times {10^{-4}}$ & $1.09 \times {10^{-1}}$ & 34\\
Hausdorff & 89.01 & $1.53 \times {10^{-4}}$ & $1.98 \times {10^{-2}}$ & 38\\
\bottomrule 
\end{tabular}
\centerline{(b) Addition attack on ModelNet40}
\newline
\newline
\begin{tabular}{l|c|cc|c}
\toprule
& Success Rate & Chamfer Distance & Hausdorff Distance & \# Points\\
\midrule
Chamfer & 96.69 & $1.89 \times {10^{-4}}$ & $6.51 \times {10^{-2}}$ & 42\\
Hausdorff & 91.72 & $1.12 \times {10^{-4}}$ & $1.15 \times {10^{-2}}$ & 34\\
\bottomrule 
\end{tabular}
\centerline{(c) Perturbation attack on ScanObjectNN}
\newline
\newline
\begin{tabular}{l|c|cc|c}
\toprule
& Success Rate & Chamfer Distance & Hausdorff Distance & \# Points\\
\midrule 
Chamfer & 97.87 & $1.99 \times {10^{-4}}$ & $7.27 \times {10^{-2}}$ & 37\\
Hausdorff & 90.44 & $1.08 \times {10^{-4}}$ & $1.10 \times {10^{-2}}$ & 38\\
\bottomrule
\end{tabular}
\centerline{(d) Addition attack on ScanObjectNN}
\caption{Attack performance of distance method on ModelNet40 and ScanObjectNN.}
\label{table:distance_method}
\end{center}%
\end{table*}

\begin{figure*}[t!]
\centering
\includegraphics[width=0.8\linewidth]{figures/obj_lambda.jpeg}
\caption{Adversarial examples generated using different settings.}
\label{fig:lambda_example}
\end{figure*}

\section{Ablation Studies}
\label{sec:AblationStudy}

\subsection{Sparsity vs Perceptibility}

\noindent We performed an in-depth analysis of our formulation by studying its constituting components. In particular, we investigated the role of the sparsity term, i.e., $\| \mathbf{\hat{a}} \|_1$, and the perceptibility term, i.e., $D(P,P')$, in Eq.~(8) in our paper. In this experiment, we set $\lambda_1$ and $\lambda_2$ to 0, respectively, and measured the corresponding performances of attacks. 

We report the performance of our method in terms of the success rate (of attack), the Chamfer distances and Hausdorff distances of generated samples to original samples, and the average numbers of points used in point perturbation and point addition in Table~\ref{table:Lambda_variation}. 

As shown in our experimental results, when the sparsity is not considered, i.e., $\lambda_1 = 0$, the adversarial generation method achieves higher attack rates but requires considerably high numbers of points. In contrast, when the perceptibility is not used, i.e., $\lambda_2 = 0$, relatively lower success rates are incurred (compared with $\lambda_1=0$), much lesser numbers of points are used but adversarial examples much deform from original point clouds (as shown in the Hausdorff distances). This phenomenon can be explained by the following imaginary experiment: take a few (even one) points on an input point cloud and move those points much away from the original point cloud. It is obvious to see that this perturbation will significantly change the shape of the point cloud and thus will affect any point cloud classification methods. However, such extreme samples can also be detected easily by using outlier or noise removal methods, e.g.,~\cite{Daniel-attack-and-defense1-2019}.

In the current implementation of our adversarial attack, we set $\lambda_1 = 0.15$ and $\lambda_2 = 50$. We notice on the difference in the values of $\lambda_1$ and $\lambda_2$, which is caused by the difference in the range of values of their associated terms. In particular, $\| \mathbf{\hat{a}} \|_1$ captures the number of manipulated points, which varies in $[0, 1024]$ while $D(P,P') \in [0,1]$ since point clouds are normalised into $[0,1]$ before being processed. We empirically observed minor changes in the attack performance of our method for $\lambda_1 \in [0.1, 0,2]$ and $\lambda_2 \in [30, 50]$ while the current settings gave the best balance for many contradictory criteria including minimal attack, high success rate, and reasonable perceptibility. We show several results illustrating the effects of the sparsity and perceptibility of adversarial examples in Figure~\ref{fig:lambda_example}.

\begin{figure*}[t!]
\centering
\includegraphics[width=0.8\linewidth]{figures/obj_ch_h.jpeg}
\caption{Chamfer Distance vs Hausdorff Distance.}
\label{fig:compare_haousdorff_chamfer}
\end{figure*}

\subsection{Chamfer Distance vs Hausdorff Distance}

\noindent We experimented our method with Chamfer and Hausdorff distance, i.e., replacing $D(P,P')$ by $D_{Chamfer}(P,P')$ and $D_{Hausdorff}(P,P')$, respectively in Eq.~(4) and Eq.~(5) in our paper. Table~\ref{table:distance_method} shows attack results of these two distance metrics in point perturbation and point addition attack. Note that the two columns labelled as ``Chamfer Distance'' and ``Hausdorff Distance'' in Table~\ref{table:distance_method} report the Chamfer and Hausdorff distances from generated adversarial examples to original point clouds. As shown in the results, there is little difference in the numbers of manipulated points between Chamfer and Hausdorff distance in both point perturbation and point addition attack. On one hand, Chamfer distance shows higher success rate. On the other hand, Hausdorff distance better preserves the perceptibility of point clouds during point manipulation.

We visually show adversarial examples generated by using Chamfer distance and Hausdorff distance in Figure~\ref{fig:compare_haousdorff_chamfer}. We qualitatively observed that attacks using Chamfer distance often place a few points far away from original point clouds, making high success rate but low perceptibility. In addition, we empirically found that adversarial examples, whose Hausdorff distance to their original point clouds is over 0.01, often include obvious outliers and thus are detectable easily. However, a comprehensive user-study on human perception of adversarial examples would better reflect the perceptibility of these distance metrics, and thus is worthwhile for future research.

\begin{table*}[t]
\small
\begin{center}
\begin{tabular}{l|c|cc|c}
\toprule
& Success Rate & Chamfer Distance & Hausdorff Distance & \# Points\\
\midrule
Critical points & 90.07 & $1.06 \times {10^{-4}}$ & $1.03 \times {10^{-2}}$ & 30\\
Using all points & 92.67 & $1.22 \times {10^{-4}}$ & $1.16 \times {10^{-2}}$ & 65\\
Ours (random points) & 90.44 & $1.08 \times {10^{-4}}$ & $1.10 \times {10^{-2}}$ & 38\\
\bottomrule 
\end{tabular}
\caption{Point addition attack performance with different point initialisation strategies on ScanObjectNN.}
\label{table:various_initialization_addition_obj_bg}
\end{center}
\end{table*}

\subsection{Initialisation of Point Selection}

\noindent Similarly to point perturbation attacks presented in our paper, we experimented point addition attacks with different initialisation schemes for point selection including: critical points-based
initialisation (i.e., using critical points from~\cite{qi2017pointnet} to initialise added points), all points-based initialisation (i.e., considering all points in a point cloud as added points), and random points-based initialisation.

We report the performance of these initialisation schemes in Table~\ref{table:various_initialization_addition_obj_bg}. Our results show that, like point perturbation, compared with critical points-based initialisation and all points-based initialisation, random points-based initialisation balance the success rate and number of points while ensuring the perceptability of adversarial examples.

\section{Visual Results of Point Addition}
\label{sec:PointAddition}

\noindent In our paper, we present visual results of our proposed point perturbation attack method and existing methods on ModelNet40 dataset. In this section, we qualitatively compare adversarial point clouds generated by our point addition attack algorithm and existing ones on ModelNet40 dataset. Figure~\ref{fig:addition_modelnet40} show several results of adversarial point clouds using point addition.

\section{Attack Performance on Real-World Data}
\label{sec:Realworld}
\begin{table*}[t]
\begin{center}
\begin{tabular}{l|c|cc|c}
\toprule
Variant & Success Rate & Chamfer Distance & Hausdorff Distance & \# Points\\
\midrule
OBJ\_BG & 91.72 & $1.12 \times {10^{-4}}$ & $1.15 \times {10^{-2}}$ & 34\\
PB\_T25 & 94.04 & $9.74 \times {10^{-4}}$ & $1.12 \times {10^{-2}}$ & 33\\
PB\_T25\_R & 91.09 & $9.53 \times {10^{-5}}$ & $1.02 \times {10^{-2}}$ & 31\\
PB\_T50\_R & 90.58 & $8.59 \times {10^{-5}}$ & $9.61 \times {10^{-3}}$ & 30\\
PB\_T50\_RS & 91.92 & $7.68 \times {10^{-5}}$ & $8.77 \times {10^{-3}}$ & 27\\
\bottomrule
\end{tabular}
\centerline{(a) Point Perturbation}
\newline
\newline
\begin{tabular}{l|c|cc|c}
\toprule
Variant & Success Rate & Chamfer Distance & Hausdorff Distance & \# Points\\
\midrule
OBJ\_BG & 90.44 & $1.08 \times {10^{-4}}$ & $1.10 \times {10^{-2}}$ & 38\\
PB\_T25 & 93.62 & $1.13 \times {10^{-4}}$ & $1.26 \times {10^{-2}}$ & 36\\
PB\_T25\_R & 92.13 & $9.06 \times {10^{-5}}$ & $9.76 \times {10^{-3}}$ & 34\\
PB\_T50\_R & 92.29 & $8.18 \times {10^{-5}}$ & $9.24 \times {10^{-3}}$ & 32\\
PB\_T50\_RS & 92.43 & $7.51 \times {10^{-5}}$ & $8.73 \times {10^{-3}}$ & 30\\
\bottomrule
\end{tabular}
\centerline{(b) Point Addition}
\caption{Attack performance to PointNet on entire ScanObjectNN.}
\label{table:entire_ScanObjectNN}
\end{center}
\end{table*}

\noindent We also evaluated our method on the entire real-world dataset, ScanObjectNN. Recall that ScanObjectNN has five variants corresponding to five challenges. Specifically, ``OBJ\_BG'' includes objects with background, ``PB\_T25'' includes objects translated by 25\%, post-fixes ``R'' and ``S'' denote rotated and scaled objects, respectively. Readers are referred to ~\cite{Mikaela-real-world-dataset-2019} for more details of ScanObjectNN dataset. 

We report the attack performance of our method to PointNet on the entire ScanObjectNN dataset in Table ~\ref{table:entire_ScanObjectNN}. As shown in results, our method maintains a success rate of more than 90\% by using only 4\% of total points. Our method also performs consistently across all the variants of ScanObjectNN. Furthermore, we observe that, amongst all the variants, OBJ\_BG appears to be the most challenging one (i.e., low success rate and high level of deformation, as shown in Hausdorff distances). This observation is also consistent with conclusion from~\cite{Mikaela-real-world-dataset-2019}, indicating that OBJ\_BG is the most difficult variant for object recognition. 

\begin{figure*}[t!]
\centering
\includegraphics[width=\linewidth]{figures/modelnet_addition.png}
\caption{Adversarial examples of point addition attack on ModelNet40. Added points are highlighted in red.}
\label{fig:addition_modelnet40}
\end{figure*}

\begin{figure*}[t!]
\centering
\includegraphics[width=\linewidth]{figures/obj_bg_addition.jpeg}
\caption{Adversarial examples of point addition attack on OBJ\_BG. Added points are highlighted in red.}
\label{fig:addition_obj_bg}
\end{figure*}

\begin{figure*}[t!]
\centering
\includegraphics[width=\linewidth]{figures/total_scan_ob.jpeg}
\caption{Adversarial examples of point perturbation attack on ScanObjectNN. Perturbed points are highlighted in red.}
\label{fig:perturbation_obj_bg}
\end{figure*}

We show several adversarial results of our method on the OBJ\_BG variant and entire ScannObjectNN dataset in Figure~\ref{fig:addition_obj_bg} and Figure~\ref{fig:perturbation_obj_bg} respectively. In general, compared with adversarial samples generated by existing attack methods, our adversarial samples look more natural; our perturbed and added points visually look like common noise and thus are hard to be noticed. This suggests the necessity to validate attack techniques in extreme situations, e.g., attacks with minimal manipulation.

\section{Defense}
\label{sec:Defense}

\begin{table*}[t]
\begin{center}

\begin{tabular}{c|l|c|c|c}
& Attack method & Outlier removal~\cite{Daniel-attack-and-defense1-2019} & Salient point removal~\cite{Daniel-attack-and-defense1-2019} & DUP-Net~\cite{Zhou-2019-ICCV} \\
\hline
\multirow{8}{*}{\rotatebox[origin=c]{90}{Perturbation}} & ~\cite{chong-first-adv-2019} Xiang et al & 85.32 & 80.77 & 78.92 \\
\cline{2-5}
& ~\cite{Daniel-attack-and-defense2-2019} stick & 23.00 & 15.40 & 39.81 \\
& ~\cite{Daniel-attack-and-defense2-2019} sink & 18.60 & 12.30 & 36.85 \\
\cline{2-5}
& ~\cite{Matthew-Robustness-map-2019} random & 84.58 & 78.41 & 69.82 \\
& ~\cite{Matthew-Robustness-map-2019} critical & 72.71 & 64.49 & 53.25 \\
\cline{2-5}
& ~\cite{Zheng-saliency-map-2019} critical & 88.65 & 88.00 & 73.08 \\
& ~\cite{Zheng-saliency-map-2019} low-score & 88.66 & 85.86 & 71.7 \\
& ~\cite{Zheng-saliency-map-2019} high-score & 77.16 & 72.06 & 64.17 \\
\cline{2-5}
& Ours & 95.55 & 95.4 & 82.21 \\
\hline
\multirow{6}{*}{\rotatebox[origin=c]{90}{Addition}} & ~\cite{chong-first-adv-2019} Xiang et al & 93.21 & 96.05 & 87.31 \\
\cline{2-5}
& ~\cite{Matthew-Robustness-map-2019} random & 77.67 & 87.25 & 68.87 \\
& ~\cite{Matthew-Robustness-map-2019} critical & 80.52 & 87.95  & 70.31 \\
\cline{2-5}
& ~\cite{Zheng-saliency-map-2019} critical & 80.10 & 88.83 & 69.5 \\
& ~\cite{Zheng-saliency-map-2019} low-score & 82.95 & 87.48 & 68.76 \\
& ~\cite{Zheng-saliency-map-2019} high-score & 70.65 & 84.52 & 66.74 \\
\cline{2-5}
& Ours & 94.21 & 96.31 & 82.28 \\
\hline
\end{tabular}
\centerline{(a) ModelNet40}
\newline

\begin{tabular}{c|l|c|c|c}
& Attack method & Outlier removal~\cite{Daniel-attack-and-defense1-2019} & Salient point removal~\cite{Daniel-attack-and-defense1-2019} & DUP-Net~\cite{Zhou-2019-ICCV} \\
\hline
\multirow{8}{*}{\rotatebox[origin=c]{90}{Perturbation}} & ~\cite{chong-first-adv-2019} Xiang et al & 86.29 & 81.14 & 80.48 \\
\cline{2-5}
& ~\cite{Daniel-attack-and-defense2-2019} stick & 26.50 & 13.70 & 49.72  \\
& ~\cite{Daniel-attack-and-defense2-2019} sink & 50.40 & 25.80 & 31.83 \\
\cline{2-5}
& ~\cite{Matthew-Robustness-map-2019} random & 86.59 & 86.21 & 74.61 \\
& ~\cite{Matthew-Robustness-map-2019} critical & 74.47 & 68.79 & 65.95\\
\cline{2-5}
& ~\cite{Zheng-saliency-map-2019} critical & 89.75 & 91.52 & 78.44\\
& ~\cite{Zheng-saliency-map-2019} low-score & 88.68 & 92.83 & 75.84\\
& ~\cite{Zheng-saliency-map-2019} high-score & 84.81 & 80.74 & 76.66\\
\cline{2-5}
& Ours & 94.32 & 96.64 & 83.64 \\
\hline
\multirow{6}{*}{\rotatebox[origin=c]{90}{Addition}} & ~\cite{chong-first-adv-2019} Xiang et al & 92.28 & 89.82 & 84.79 \\
\cline{2-5}
& ~\cite{Matthew-Robustness-map-2019} random & 82.17 & 91.47 & 75.39 \\
& ~\cite{Matthew-Robustness-map-2019} critical & 87.24 & 90.53 & 77.36\\
\cline{2-5}
& ~\cite{Zheng-saliency-map-2019} critical & 84.50 & 92.64 & 76.74\\
& ~\cite{Zheng-saliency-map-2019} low-score & 87.55 & 92.08 & 75.09 \\
& ~\cite{Zheng-saliency-map-2019} high-score & 82.33 & 88.35 & 76.30\\
\cline{2-5}
& Ours & 93.12 & 96.56 & 83.54 \\
\hline
\end{tabular}
\centerline{(b) OBJ\_BG}

%\vspace{0.02cm}
\caption{Attack to defense of different attack methods.}
\label{table:attack_to_defense}
\end{center}
\end{table*}

\begin{table*}[t]
\begin{center}
\begin{tabular}{c|c|c|c|c}
\toprule
& Success rate & Outlier removal~\cite{Daniel-attack-and-defense1-2019} & Salient point removal~\cite{Daniel-attack-and-defense1-2019} & DUP-Net~\cite{Zhou-2019-ICCV} \\
\midrule
ModelNet40 & 89.38 & 95.55 & 95.40 & 82.21\\
OBJ\_BG & 91.72 & 94.32 & 96.64 & 83.64\\
PB\_T25 & 94.04 & 91.83 & 93.72 & 81.73\\
PB\_T25\_R & 91.09 & 91.00 & 93.81 & 81.98\\
PB\_T50\_R & 90.58 & 90.35 & 93.49 & 79.47\\
PB\_T50\_RS & 91.92 & 89.13 & 93.35 & 81.27\\
\bottomrule 
\end{tabular}
\centerline{(a) Perturbation}
\newline
\newline
\begin{tabular}{c|c|c|c|c}
\toprule
& Success rate & Outlier removal~\cite{Daniel-attack-and-defense1-2019} & Salient point removal~\cite{Daniel-attack-and-defense1-2019} & DUP-Net~\cite{Zhou-2019-ICCV} \\
\midrule
ModelNet40 & 89.01 & 94.21 & 96.31 & 82.28\\
OBJ\_BG & 90.44 & 93.12 & 96.56 & 83.54\\
PB\_T25 & 93.62 & 90.34 & 94.24 & 82.59\\
PB\_T25\_R & 92.13 & 89.31 & 94.34 & 81.64\\
PB\_T50\_R & 92.29 & 88.68 & 93.50 & 80.0\\
PB\_T50\_RS & 92.43 & 87.79 & 93.50 & 81.52\\
\bottomrule
\end{tabular}
\centerline{(b) Addition}
\caption{Attack to defense of our method to PointNet.}
\label{table:attack_to_defense_PointNet}
\end{center}%
\end{table*}

\noindent We experimented adversarial defense techniques to our adversarial point clouds. In this experiment, we implemented two defense algorithms in~\cite{Daniel-attack-and-defense1-2019}: outlier removal and salient point removal, and DUP-NET in~\cite{Zhou-2019-ICCV}. The outlier removal technique first estimates statistical outliers from an input point set and then removes points that have large standard deviations. The salient point removal operates by first estimating point saliency and then removing points in the order from high to low saliency. DUP-NET makes use of a similar strategy with removal outlier. However, it applies upsampling after removal outlier.

We show defense results in Table~\ref{table:attack_to_defense}. In general, it is moderately easy to defend adversarial point clouds using the above methods, with a success rate up to 94\% for adversarial examples in ModelNet40. Despite that, we found defense on real-world data is less effective, e.g., the success rate decreases on the hardest variant of ScanObjectNN. In addition, the defenses are also not effective to structured manipulation such as adding particular shapes like stick/sink in~\cite{Daniel-attack-and-defense2-2019}.

We further experimented the defense algorithms in~\cite{Daniel-attack-and-defense1-2019} to PointNet on all variants of ScanObjectNN dataset (see Table~\ref{table:attack_to_defense_PointNet}). Experimental results show that the salient point removal method works pretty well in cases of severe object deformations, e.g., the variants PB\_50\_R and PB\_50\_RS. This is because points added by the point addition attack could be close to salient points and thus noticed by the salient point removal method. It would also be useful to study how to make adversarial examples with minimal attacks on salient points.

\section{Transferability}
\label{sec:Transfer}

\noindent In this experiment, we investigated the transferability of adversarial examples across different point cloud networks. Specifically, we fed adversarial point clouds generated with PointNet~\cite{qi2017pointnet} as the target network to  PointNet++~\cite{qi2017pointnet++} for attacks. In the opposite way, we transferred adversarial examples generated using PointNet++ to PointNet. 

We report the success rates of cross-network adversarial example transfers for both point perturbation and point addition on ModelNet40 and OBJ\_BG of ScanObjectNN in Table~\ref{table:transfer_attack}. We found that both point perturbation and point addition attack are challenging to cross-network transfers. For instance, the attack success rates in both ways: PointNet to PointNet++ and PointNet++ to PointNet, are about 20\% on both ModelNet40 and OBJ\_BG. This observation is also consistent to that by Xiang et al.~\cite{chong-first-adv-2019}.

\begin{table}[t]
\begin{center}
\begin{tabular}{l|c|c}
\toprule
& Point Perturbation & Point Addition\\
\midrule
ModelNet40 & 7.68 & 6.49\\
OBJ\_BG & 25.75 & 25.11\\
\bottomrule
\end{tabular}
\centerline{(a) PointNet to PointNet++}
\newline
\newline
\begin{tabular}{l|c|c}
\toprule
& Point Perturbation & Point Addition\\
\midrule
ModelNet40 & 25.66 & 22.34\\
OBJ\_BG & 19.55 & 20.94\\
\bottomrule
\end{tabular}
\centerline{(b) PointNet++ to PointNet}
\end{center}%
\caption{Cross-network adversarial example transfer. While the success rates are low, the results suggest that real-world data is more vulnerable to black box attacks.}
\label{table:transfer_attack}
\end{table}

\begin{table*}[t]
\begin{center}
\begin{tabular}{l|c|cc|c}
\toprule
Method & Success Rate & Chamfer Distance & Hausdorff Distance & \# Points\\
\hline
~\cite{Matthew-Robustness-map-2019} random & ~7.05 & ~$9.89\times10^{-4}$ & $3.99\times10^{-2}$ & 85 \\
%\hline
~\cite{Matthew-Robustness-map-2019} critical & 95.05 & $152\times10^{-4}$ & $8.82\times10^{-2}$ & 107 \\
\hline
~\cite{Zheng-saliency-map-2019} critical & 59.82 &  $113\times10^{-4}$ & $18.70\times10^{-2}$ & 400 \\
%\hline
~\cite{Zheng-saliency-map-2019} low-score & ~4.16 & $62.90\times10^{-4}$ & $11.40\times10^{-2}$ & 400 \\
%\hline
~\cite{Zheng-saliency-map-2019} high-score & 82.11 & $91.30\times10^{-4}$ & $15.70\times10^{-2}$ & 400 \\
\hline 
Ours (point perturbation) & 89.38 &  \textbf{$1.55\times10^{-4}$} & \textbf{$1.88\times10^{-2}$} & 36 \\
Ours (point addition) & 89.01 &  \textbf{$1.53\times10^{-4}$} & \textbf{$1.98\times10^{-2}$} & 38 \\
\hline
\end{tabular}
\centerline{(a) ModelNet40}
\newline

\begin{tabular}{l|c|cc|c}
\toprule
Method & Success Rate & Chamfer Distance & Hausdorff Distance & \# Points\\
\hline
~\cite{Matthew-Robustness-map-2019} random & ~4.96 & ~$9.05\times10^{-4}$ & $2.02\times10^{-2}$ & 23 \\
%\hline
~\cite{Matthew-Robustness-map-2019} critical & 71.87 & $119\times10^{-4}$ & $11.40\times10^{-2}$ & 320 \\
\hline
~\cite{Zheng-saliency-map-2019} critical & 43.50 &  $118\times10^{-4}$ & $21\times10^{-2}$ & 400 \\
%\hline
~\cite{Zheng-saliency-map-2019} low-score & ~2.60 & $74\times10^{-4}$ & $13.90\times10^{-2}$ & 400 \\
%\hline
~\cite{Zheng-saliency-map-2019} high-score & 77.78 & $101\times10^{-4}$ & $18.40\times10^{-2}$ & 400 \\
\hline
Ours (point perturbation) & 91.72 &  \textbf{$1.12\times10^{-4}$} & \textbf{$1.15\times10^{-2}$} & 34 \\
Ours (point addition) & 90.44 &  \textbf{$1.08\times10^{-4}$} & \textbf{$1.10\times10^{-2}$} & 38 \\
\hline
\end{tabular}
\centerline{(b) OBJ\_BG}

\caption{Comparison of our adversarial attack methods with existing point removal attack methods.}
\label{table:removal_attack}
\end{center}
\end{table*}

An interesting observation from experimental results is that real-world adversarial examples in ScanObjectNN are easier to transfer than synthetic examples in ModelNet40, which makes real-world data more vulnerable to black box attacks. This also suggests the need to further enhance the robustness of 3D point cloud networks.

\section{Comparison with Point Removal}
\label{sec:comparison}

\noindent In our paper, we applied the point selection strategies in~\cite{Matthew-Robustness-map-2019} and~\cite{Zheng-saliency-map-2019} but replaced the point removal procedure in those methods by point perturbation and point addition operation for fair comparison with other adversarial attacks where only point perturbation and point addition are used. 

In this section, we provide the performance of~\cite{Matthew-Robustness-map-2019} and~\cite{Zheng-saliency-map-2019} with point removal\footnote{We re-implemented these methods.} and compare these methods with our point perturbation and point addition attacks. We report the results of this experiment in Table~\ref{table:removal_attack}. 

\section{Detailed Derivations}
\label{sec:iterative}

\noindent Recall that our adversarial examples are generated by minimising the objective function $f(P,\mathbf{\hat{a}}, E)$ defined in Eq.~(8) in the paper. To solve this problem, we applied the iterative gradient descent methods in~\cite{goodfellow-fgsm-iclr14}, which incrementally updates $\hat{a}_i$ and $\mathbf{e}_i$ as follows:
\begin{align*}
\hat{a}_i^{(n+1)} = \hat{a}_i^{(n)} - \gamma \frac{\partial f}{\partial \hat{a}_i}\\
\mathbf{e}_i^{(n+1)} = \mathbf{e}_i^{(n)} - \gamma \frac{\partial f}{\partial \mathbf{e}_i}
\end{align*}
where $(\hat{a}_i^{(n)},\mathbf{e}_i^{(n)})$ is the solution at the $n$-th step and $\gamma$ is set to 0.01 in our implementation.

We derive the partial derivatives $\frac{\partial f}{\partial \hat{a}_i}$ and $\frac{\partial f}{\partial \mathbf{e}_i}$ as follows:
\begin{align*}
\frac{\partial f}{\partial \hat{a}_i} &= \lambda_1 + \lambda_2\frac{\partial D(P,P')}{\partial \hat{a}_i} + \frac{\partial h(P')}{\partial \hat{a}_i}\\
\frac{\partial f}{\partial \mathbf{e}_i} &= \lambda_2\frac{\partial D(P,P')}{\partial \mathbf{e}_i} + \frac{\partial h(P')}{\partial \mathbf{e}_i}
\end{align*}

It can be seen that the calculations of $\frac{\partial f}{\partial \hat{a}_i}$ and $\frac{\partial f}{\partial \mathbf{e}_i}$ require $\frac{\partial D(P,P')}{\partial \hat{a}_i}$, $\frac{\partial D(P,P')}{\partial \mathbf{e}_i}$, $\frac{\partial h(P')}{\partial \hat{a}_i}$, and $\frac{\partial h(P')}{\partial \mathbf{e}_i}$. 

First, we present the calculations of $\frac{\partial D(P,P')}{\partial \hat{a}_i}$ and $\frac{\partial D(P,P')}{\partial \mathbf{e}_i}$. As shown in our paper, we propose two ways to realise $D(P,P')$: using Chamfer distance and Hausdorff distance. For convenience in calculations, we rewrite $D(P,P')$ as follows,
\begin{align*}
D(P,P') = \max \bigg\{ D(P \rightarrow P'), 
D(P' \rightarrow P) \bigg\}
\end{align*}
where, depending on the distance metric used, $D(P \rightarrow P')$ and $D(P' \rightarrow P)$ can be defined as,
\begin{align*}
D_{Chamfer}(P \rightarrow P') &= \frac{1}{|P|} \sum_{\mathbf{p}_i \in P} \min_{\mathbf{p}'_j \in P'} \Vert \mathbf{p}_i - \mathbf{p}'_j \Vert_2 \\
D_{Chamfer}(P' \rightarrow P) &= \frac{1}{|P'|} \sum_{\mathbf{p}'_j \in P'} \min_{\mathbf{p}_i \in P} \Vert \mathbf{p}'_j - \mathbf{p}_i \Vert_2 \\
D_{Hausdorff}(P \rightarrow P') &= \max_{\mathbf{p}_i \in P} \min_{\mathbf{p}'_j \in P'} \Vert \mathbf{p}_i - \mathbf{p}'_j \Vert_2 \\
D_{Hausdorff}(P' \rightarrow P) &= \max_{\mathbf{p}'_j \in P} \min_{\mathbf{p}_i \in P} \Vert \mathbf{p}'_j - \mathbf{p}_i \Vert_2
\end{align*}

Next, we obtain,
\begin{align*}
\frac{\partial D(P,P')}{\partial \hat{a}_i}
&= \begin{cases} \frac{\partial D(P \rightarrow P')}{\partial \hat{a}_i} &\mbox{if } D(P \rightarrow P') \geq D(P' \rightarrow P) \\
\frac{\partial D(P' \rightarrow P)}{\partial \hat{a}_i} & \mbox{otherwise} \end{cases}\\
\frac{\partial D(P,P')}{\partial \mathbf{e}_i}
&= \begin{cases} \frac{\partial D(P \rightarrow P')}{\partial \mathbf{e}_i} &\mbox{if } D(P \rightarrow P') \geq D(P' \rightarrow P) \\
\frac{\partial D(P' \rightarrow P)}{\partial \mathbf{e}_i} & \mbox{otherwise} \end{cases}
\end{align*}

For Chamfer distance, we have,
\begin{align*}
\frac{\partial D_{Chamfer}(P \rightarrow P')}{\partial \hat{a}_i}
&= \frac{1}{|P|} \sum_{p_k \in P} \frac{\partial}{\partial \hat{a}_i}(\min_{\mathbf{p}'_j \in P'}\Vert \mathbf{p}_k - \mathbf{p}'_j \Vert_2) \\
\frac{\partial D_{Chamfer}(P \rightarrow P')}{\partial \mathbf{e}_i}
&= \frac{1}{|P|} \sum_{p_k \in P} \frac{\partial}{\partial \mathbf{e}_i}(\min_{\mathbf{p}'_j \in P'}\Vert \mathbf{p}_k - \mathbf{p}'_j \Vert_2)
\end{align*}
where
\begin{align*}
&\frac{\partial}{\partial \hat{a}_i}(\min_{\mathbf{p}'_j \in P'}\Vert \mathbf{p}_k - \mathbf{p}'_j \Vert_2) \\
&= \begin{cases} \frac{\mathbf{e}_i^{\top}(\mathbf{p}'_i - \mathbf{p}_k)}{\Vert \mathbf{p}'_i - \mathbf{p}_k \Vert_2} & \mbox{if } \mathbf{p}'_i = \underset{\mathbf{p}'_j \in P'}{\operatorname{argmin}} \Vert \mathbf{p}_k - \mathbf{p}'_j \Vert_2 \\
0 & \mbox{otherwise} \end{cases}\\
&\frac{\partial}{\partial \mathbf{e}_i}(\min_{\mathbf{p}'_j \in P'}\Vert \mathbf{p}_k - \mathbf{p}'_j \Vert_2) \\
&= \begin{cases} \frac{\hat{a}_i (\mathbf{p}'_i - \mathbf{p}_k)}{\Vert \mathbf{p}'_i - \mathbf{p}_k \Vert_2}  &\mbox{if } \mathbf{p}'_i = \underset{\mathbf{p}'_j \in P'}{\operatorname{argmin}} \Vert \mathbf{p}_k - \mathbf{p}'_j \Vert_2 \\
0 & \mbox{otherwise} \end{cases}
\end{align*}

For Hausdorff distance, we have,
\begin{align*}
&\frac{\partial D_{Hausdorff}(P \rightarrow P')}{\partial \hat{a}_i}\\
&= \begin{cases} \frac{\mathbf{e}_i^{\top} (\mathbf{p}'_i - \mathbf{p}_k)}{\Vert \mathbf{p}'_i - \mathbf{p}_k \Vert_2}  &\mbox{if } \Vert \mathbf{p}_k - \mathbf{p}'_i \Vert_2 = \underset{\mathbf{p}_l \in P}{\max} \underset{\mathbf{p}'_j \in P'}{\min} \Vert \mathbf{p}_l - \mathbf{p}'_j \Vert_2 \\
0 & \mbox{otherwise} \end{cases}\\
&\frac{\partial D_{Hausdorff}(P \rightarrow P')}{\partial \mathbf{e}_i}\\
&= \begin{cases} \frac{\hat{a}_i (\mathbf{p}'_i - \mathbf{p}_k)}{\Vert \mathbf{p}'_i - \mathbf{p}_k \Vert_2}  &\mbox{if } \Vert \mathbf{p}_k - \mathbf{p}'_i \Vert_2 = \underset{\mathbf{p}_l \in P}{\max} \underset{\mathbf{p}'_j \in P'}{\min} \Vert \mathbf{p}_l - \mathbf{p}'_j \Vert_2 \\
0 & \mbox{otherwise} \end{cases}
\end{align*}

We note that $\frac{\partial D_{Chamfer}(P' \rightarrow P)}{\partial \hat{a}_i}$,  $\frac{\partial D_{Chamfer}(P' \rightarrow P)}{\partial \mathbf{e}_i}$, $\frac{\partial D_{Hausdorff}(P' \rightarrow P)}{\partial \hat{a}_i}$,  $\frac{\partial D_{Hausdorff}(P' \rightarrow P)}{\partial \mathbf{e}_i}$ can be calculated similarly.

Finally, we compute $\frac{\partial h(P')}{\partial \hat{a}_i}$ and $\frac{\partial h(P')}{\partial \mathbf{e}_i}$ as follows,
\begin{align*}
\frac{\partial h(P')}{\partial \hat{a}_i} &= \frac{\partial h(P')}{\partial \mathbf{p}'_i}  \frac{\partial \mathbf{p}'_i}{\partial \hat{a}_i}=\mathbf{e}_i^{\top} \frac{\partial h(P')}{\partial \mathbf{p}'_i} \\
\frac{\partial h(P')}{\partial \mathbf{e}_i} &= \frac{\partial h(P')}{\partial \mathbf{p}'_i} \frac{\partial \mathbf{p}'_i}{\partial \mathbf{e}_i} = \hat{a}_i \frac{\partial h(P')}{\partial \mathbf{p}'_i} 
\end{align*}
where $\frac{\partial h(P')}{\partial \mathbf{p}'_i}$ is achievable from a target point cloud network. For instance, PointNet applies multi-layer perceptrons on points individually, which support the calculations of $\frac{\partial h(P')}{\partial \mathbf{p}'_i}$, for every point $\mathbf{p}'_i \in P'$.
